# Supplementary material for: Fibottention: Inceptive Visual Representation Learning with Diverse Attention Across Heads
Source: arXiv:2406.19391 source file (2026-02-12)
Supplement: Supplementary file 1 [file fig-random-attention.tex]

\begin{figure}[ht]
    \centering
    \includegraphics[width=\textwidth]{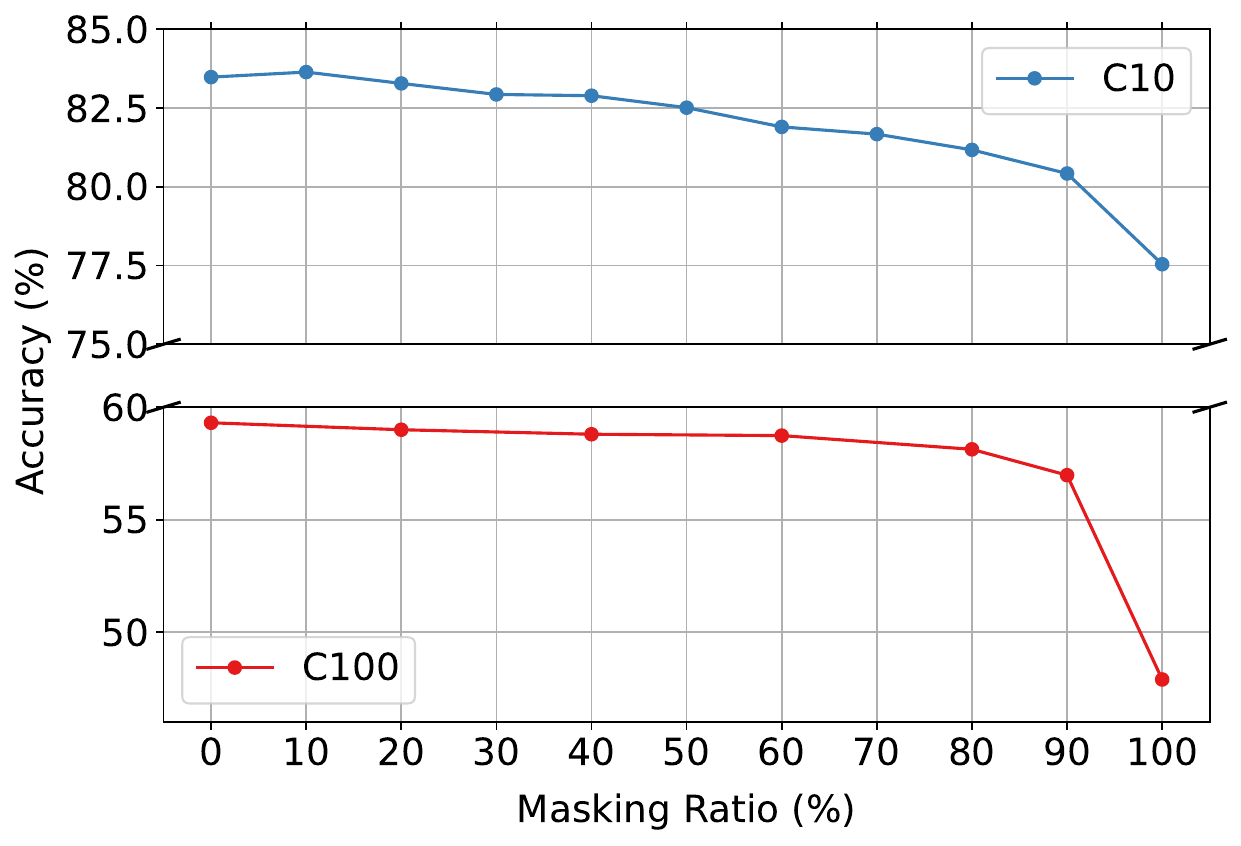}
    \caption{Performance comparison of Random Attention across the C10 and C100 datasets with varying masking ratios. Top-1 accuracy is reported.}
    \label{fig:random_masking}
\end{figure}
