# Supplementary material for: Fibottention: Inceptive Visual Representation Learning with Diverse Attention Across Heads
Source: arXiv:2406.19391 source file (2026-02-12)
Supplement: Supplementary file 2 [file fig-window-sizes.tex]

\begin{figure}[h]
    \centering
    \includegraphics[width=\textwidth]{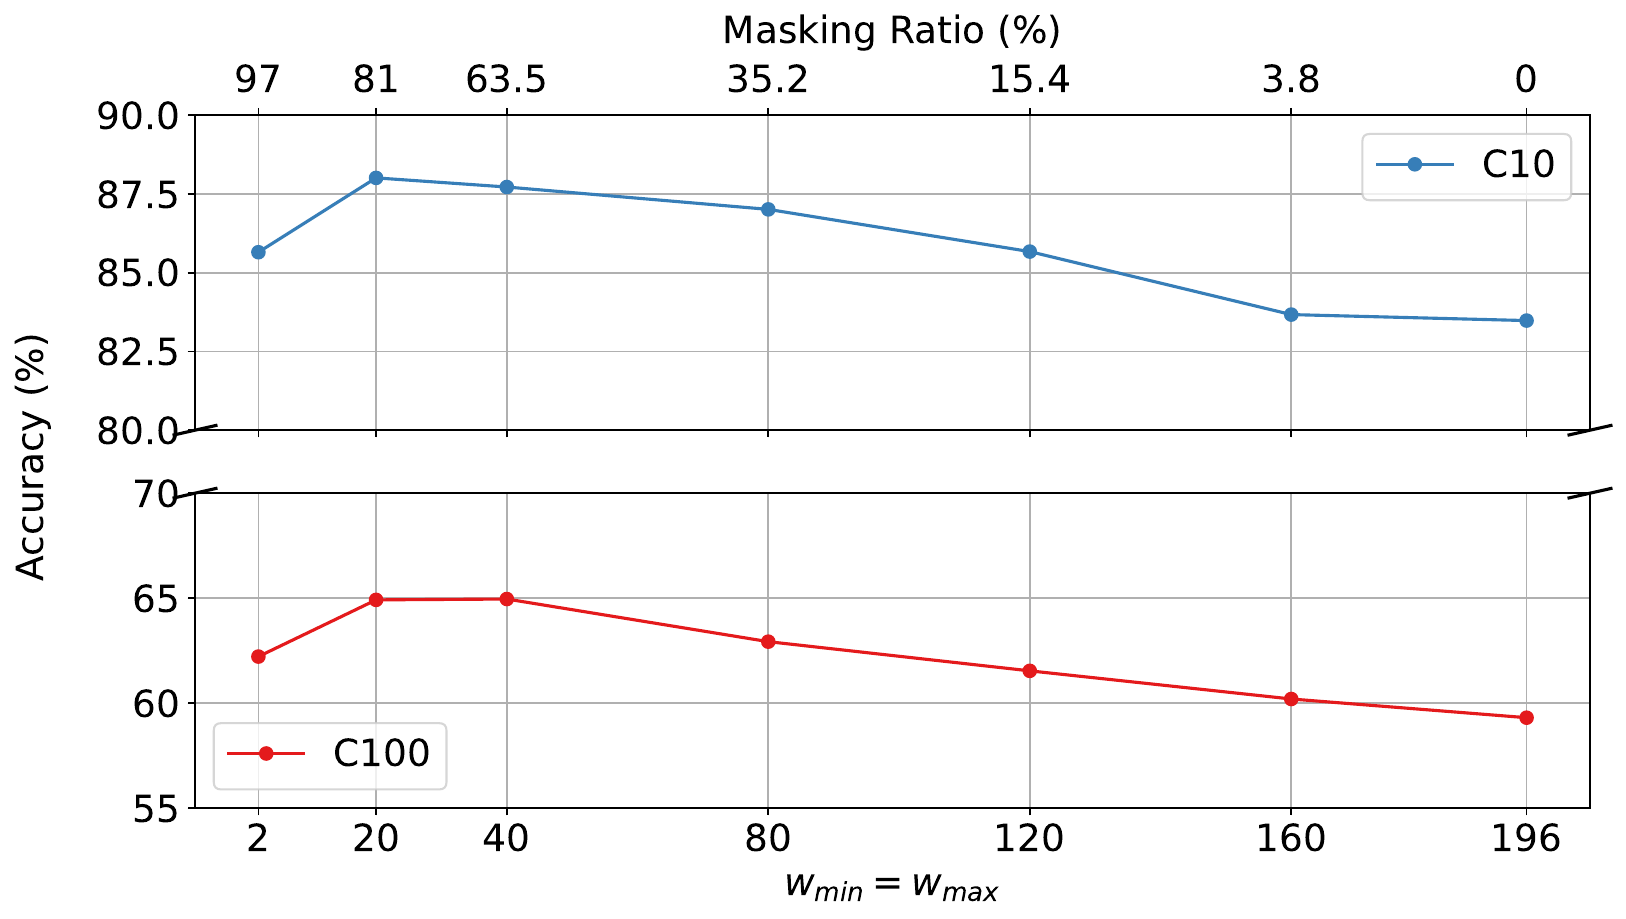}
    \caption{Top-1 accuracy of windowed self-attention on CIFAR-10~\cite{cifar} and CIFAR-100~\cite{cifar} as a function of the shared window size $w_i = \wmin = \wmax$.}
    \label{fig:window-sizes}
\end{figure}
