# Supplementary material for: Fibottention: Inceptive Visual Representation Learning with Diverse Attention Across Heads
Source: arXiv:2406.19391 source file (2026-02-12)
Supplement: Supplementary file 10 [file 03_Fibottention.tex]

\begin{algorithm}[h]
\caption{\textbf{getMask}, Generation of Sparsity Patterns of \modelname.}
\label{alg:Fibomask}
\begin{algorithmic}[1]
\State \textbf{Input:} $L,N,h,\wmin,\wmax,\text{is\_modified}$
\State \textbf{Output:} $\Omega \in \{0,1\}^{h\times (N+1)\times (N+1)}$
\State $\phi \gets \frac{1+\sqrt{5}}{2}$
\State $\Omega \gets 0^{h\times (N+1)\times (N+1)}$
\For{\textbf{each} head $i \in \{1,\cdots,h\}$}
    \State $w_i \gets \wmin$ \If{$h>1$} $+\left\lfloor \frac{(i-1)(\wmax-\wmin)}{h-1}\right\rfloor$ \EndIf
    \State $a \gets \lfloor \lfloor i\phi \rfloor \phi \rfloor,\;\; b \gets \lfloor \lfloor i \phi \rfloor\phi^2 \rfloor$ \Comment{Wythoff pair for head $i$}
    \If{$\text{is\_modified}$}
        \State $b_{\text{Wyt-m}} \gets b-a$;\;\; $a_{\text{Wyt-m}} \gets a-b_{\text{Wyt-m}}$
        \State $I \gets \textbf{getFibonacci}(a_{\text{Wyt-m}},b_{\text{Wyt-m}},w_i)$
    \Else
        \State $I \gets \textbf{getFibonacci}(a,b,w_i)$
    \EndIf

    \State $\Theta \gets 0^{(N+1)\times (N+1)}$
    \State $\Theta_{0,:}\gets 1$;\;\;$\Theta_{:,0}\gets 1$ \Comment{Keep class-token connections}
    \For{\textbf{each} $o \in I$}
        \If{$o \le 0$} \State \textbf{continue} \EndIf
        \For{\textbf{each} $j \in \{0,\cdots,N-o\}$}
            \State $(\Theta)_{j,\,j+o}\gets 1$;\;\; $(\Theta)_{j+o,\,j}\gets 1$ \Comment{Allow $\pm o$ offsets}
        \EndFor
    \EndFor
    \State $\Omega[i,:,:]\gets \Theta$
\EndFor

\State $\Omega \gets \textbf{randomshuffle}(L,\Omega)$ \Comment{Assign masks across $L$ layers}
\State \Return $\Omega$
\end{algorithmic}
\end{algorithm}
