# Supplementary material for: Fibottention: Inceptive Visual Representation Learning with Diverse Attention Across Heads
Source: arXiv:2406.19391 source file (2026-02-12)
Supplement: Supplementary file 17 [file tab-settings.tex]

\begin{table}[ht]
    \centering
    \caption{C10, C100, and Tiny-IN Training Settings~\cite{deit}.}
    \begin{tabular}{@{}l@{\hspace{8pt}}p{0.3\linewidth}@{}}
    \toprule
        Input Size & 224$\times$224 \\
        Crop Ratio & 0.9  \\
        Batch Size & 64 \\
        \midrule
        Optimizer & AdamW \\
        Optimizer Epsilon & 1.0e-06 \\
        Momentum & 0.9 \\
        Weight Decay & 0.05 \\ 
        Gradient Clip & 1.0 \\
        \midrule
        Learning Rate Schedule & Cosine\\
        Learning Rate & 1e-3 \\
        Warmup LR & 1.0e-6 \\
        Min LR & 1.0e-5 \\
        Epochs & 100 \\
        Decay Epochs & 1.0 \\
        Warmup Epochs & 5 \\
        Decay Rate & 0.988 \\
        \midrule
        Exponential Moving Average (EMA) & True \\
        EMA Decay & 0.99992 \\
        \midrule
        Random Resize \& Crop Scale \& Ratio & (0.08, 1.0),\\
        &(0.67, 1.5)\\
        Random Horizontal Flip Probability & 0.5 \\
        Color Jittering & 0.4 \\
        Auto-augmentation & rand-m15-n2-mstd1.0-inc1\\
        Mixup & True \\
        Cutmix & True \\
        Mixup, Cutmix Probability & 0.5, 0.5 \\
        Mixup Mode & Batch \\
        Label Smoothing & 0.1 \\
    \bottomrule
    \end{tabular}
    \label{tab:in1k_settings}
\end{table}
